# Supplementary material for: Bidirectional Typing with Freezing, Skeletons, and Ghosts
Source: arXiv:2607.16061 source file (2026-11-30)
Supplement: Supplementary file 1 [file appendix-labels.tex]

% Generated from the resolved full-paper auxiliary and PAX files.
% It freezes appendix reference values and joins PDF destinations.
\makeatletter
\providecommand\hyper@newdestlabel[2]{}
\newlabel{app:benchmark}{{A}{29}{Comparison of Type Systems for FCP}{appendix.A}{}}
\newlabel{app:benchmark@cref}{{[appendix][1][]A}{[1][29][]29}{}{}{}}
\newlabel{fig:comparison-table-QL}{{8}{29}{Comparison for existing examples from \citet {SerranoHVJ18,SerranoHJV20}. \yes ~means accepted, \no ~means rejected, and \half ~means accepted with freezing}{figure.caption.27}{}}
\newlabel{fig:comparison-table-QL@cref}{{[figure][8][]8}{[1][29][]29}{}{}{}}
\newlabel{fig:comparison-table-new}{{9}{30}{Comparison for the new examples}{figure.caption.28}{}}
\newlabel{fig:comparison-table-new@cref}{{[figure][9][]9}{[1][29][]30}{}{}{}}
\newlabel{fig:function-signatures}{{10}{30}{Type signatures for functions used in the comparison. For Church encodings, $\List \;a$ denotes $\forall b.b\to (a\to b\to b)\to b$}{figure.caption.29}{}}
\newlabel{fig:function-signatures@cref}{{[figure][10][]10}{[1][29][]30}{}{}{}}
\newlabel{app:decl-spec}{{B}{31}{Supplementary Specification and Metatheory for Declarative Type System}{appendix.B}{}}
\newlabel{app:decl-spec@cref}{{[appendix][2][]B}{[1][31][]31}{}{}{}}
\newlabel{app:decl-proof}{{B}{31}{Supplementary Specification and Metatheory for Declarative Type System}{appendix.B}{}}
\newlabel{app:decl-proof@cref}{{[appendix][2][]B}{[1][31][]31}{}{}{}}
\newlabel{app:all-in-one-subtyping}{{B.1}{31}{All-in-One Subtyping}{subsection.B.1}{}}
\newlabel{app:all-in-one-subtyping@cref}{{[appendix][1][2]B.1}{[1][31][]31}{}{}{}}
\newlabel{fig:decl-subtyping-all}{{11}{31}{Declarative subtyping rules for both types and skeletons}{figure.caption.30}{}}
\newlabel{fig:decl-subtyping-all@cref}{{[figure][11][]11}{[1][31][]31}{}{}{}}
\newlabel{app:syntax-directed}{{B.2}{31}{Soundness and Completeness of the Syntax-Directed Type System}{subsection.B.2}{}}
\newlabel{app:syntax-directed@cref}{{[appendix][2][2]B.2}{[1][31][]31}{}{}{}}
\newlabel{lemma:typing-syn-soundness}{{B.1}{31}{Soundness of Syntax-Directed Rule}{lemma.appendix.B.1}{}}
\newlabel{lemma:typing-syn-soundness@cref}{{[lemma][1][2]B.1}{[1][31][]31}{}{}{}}
\newlabel{lemma:typing-syn-completeness}{{B.2}{31}{Completeness of Syntax-Directed Rule}{lemma.appendix.B.2}{}}
\newlabel{lemma:typing-syn-completeness@cref}{{[lemma][2][2]B.2}{[1][31][]31}{}{}{}}
\newlabel{app:algo-spec}{{C}{32}{Full Specification for the Algorithmic Type System}{appendix.C}{}}
\newlabel{app:algo-spec@cref}{{[appendix][3][]C}{[1][32][]32}{}{}{}}
\newlabel{app:metasubstitutions}{{C.1}{32}{Metasubstitutions}{subsection.C.1}{}}
\newlabel{app:metasubstitutions@cref}{{[appendix][1][3]C.1}{[1][32][]32}{}{}{}}
\newlabel{fig:information-increase-and-equivalence}{{12}{32}{Metasubstitutions (information increase) and equivalence of metasubstitutions}{figure.caption.31}{}}
\newlabel{fig:information-increase-and-equivalence@cref}{{[figure][12][]12}{[1][32][]32}{}{}{}}
\newlabel{app:decl-in-algo-context}{{C.2}{32}{Declarative Judgements in Algorithmic Contexts}{subsection.C.2}{}}
\newlabel{app:decl-in-algo-context@cref}{{[appendix][2][3]C.2}{[1][32][]32}{}{}{}}
\newlabel{fig:declarative-in-algo-context}{{13}{33}{Declarative rules in algorithmic contexts (only showing changed rules)}{figure.caption.32}{}}
\newlabel{fig:declarative-in-algo-context@cref}{{[figure][13][]13}{[1][32][]33}{}{}{}}
\newlabel{app:algo-type-inference}{{C.3}{33}{Algorithmic Type Inference}{subsection.C.3}{}}
\newlabel{app:algo-type-inference@cref}{{[appendix][3][3]C.3}{[1][32][]33}{}{}{}}
\newlabel{fig:alg-type-inference}{{14}{34}{Algorithmic type inference and skeleton splitting}{figure.caption.33}{}}
\newlabel{fig:alg-type-inference@cref}{{[figure][14][]14}{[1][33][]34}{}{}{}}
\newlabel{app:algo-skeleton-inference}{{C.4}{34}{Algorithmic Skeleton Inference}{subsection.C.4}{}}
\newlabel{app:algo-skeleton-inference@cref}{{[appendix][4][3]C.4}{[1][34][]34}{}{}{}}
\newlabel{fig:alg-skeleton-inference}{{15}{35}{Algorithmic skeleton inference}{figure.caption.34}{}}
\newlabel{fig:alg-skeleton-inference@cref}{{[figure][15][]15}{[1][34][]35}{}{}{}}
\newlabel{thmt@@soundSkeletonInference@data}{{\def \theequation {\@arabic {\c@equation }}\def \theHequation {(restate \theHthmt@dummyctr )0}\setcounter {equation}{0}}{35}{Algorithmic Skeleton Inference}{definition.appendix.C.1}{}}
\newlabel{thmt@@soundSkeletonInference@data@cref}{{[appendix][4][3]C.4}{[1][35][]35}{}{}{}}
\newlabel{thmt@@soundSkeletonInference}{{C.2}{35}{Soundness of skeleton inference}{theorem.appendix.C.2}{}}
\newlabel{thmt@@soundSkeletonInference@cref}{{[theorem][2][3]C.2}{[1][35][]35}{}{}{}}
\newlabel{thm:sound-skeleton-inference}{{C.2}{35}{Soundness of skeleton inference}{theorem.appendix.C.2}{}}
\newlabel{thm:sound-skeleton-inference@cref}{{[theorem][2][3]C.2}{[1][35][]35}{}{}{}}
\newlabel{thmt@@completeSkeletonInference@data}{{\def \theequation {\@arabic {\c@equation }}\def \theHequation {(restate \theHthmt@dummyctr )0}\setcounter {equation}{0}}{35}{Algorithmic Skeleton Inference}{theorem.appendix.C.2}{}}
\newlabel{thmt@@completeSkeletonInference@data@cref}{{[appendix][4][3]C.4}{[1][35][]35}{}{}{}}
\newlabel{thmt@@completeSkeletonInference}{{C.3}{35}{Completeness and optimality of skeleton inference}{theorem.appendix.C.3}{}}
\newlabel{thmt@@completeSkeletonInference@cref}{{[theorem][3][3]C.3}{[1][35][]35}{}{}{}}
\newlabel{thm:complete-skeleton-inference}{{C.3}{35}{Completeness and optimality of skeleton inference}{theorem.appendix.C.3}{}}
\newlabel{thm:complete-skeleton-inference@cref}{{[theorem][3][3]C.3}{[1][35][]35}{}{}{}}
\newlabel{app:algo-subtyping}{{C.5}{35}{Algorithmic Subtyping}{subsection.C.5}{}}
\newlabel{app:algo-subtyping@cref}{{[appendix][5][3]C.5}{[1][35][]35}{}{}{}}
\newlabel{fig:alg-subtyping}{{16}{36}{Algorithmic subtyping}{figure.caption.35}{}}
\newlabel{fig:alg-subtyping@cref}{{[figure][16][]16}{[1][35][]36}{}{}{}}
\newlabel{fig:poly-info-extraction}{{17}{37}{Constraint collection}{figure.caption.36}{}}
\newlabel{fig:poly-info-extraction@cref}{{[figure][17][]17}{[1][35][]37}{}{}{}}
\newlabel{fig:constraint-solving}{{18}{38}{Constraint solving}{figure.caption.37}{}}
\newlabel{fig:constraint-solving@cref}{{[figure][18][]18}{[1][37][]38}{}{}{}}
\newlabel{app:algo-consistency}{{C.6}{38}{Algorithmic Consistency}{subsection.C.6}{}}
\newlabel{app:algo-consistency@cref}{{[appendix][6][3]C.6}{[1][38][]38}{}{}{}}
\newlabel{thmt@@soundConsistency@data}{{\def \theequation {\@arabic {\c@equation }}\def \theHequation {(restate \theHthmt@dummyctr )0}\setcounter {equation}{0}}{39}{Algorithmic Consistency}{Item.5}{}}
\newlabel{thmt@@soundConsistency@data@cref}{{[appendix][6][3]C.6}{[1][39][]39}{}{}{}}
\newlabel{thmt@@soundConsistency}{{C.6}{39}{Soundness of consistency}{lemma.appendix.C.6}{}}
\newlabel{thmt@@soundConsistency@cref}{{[lemma][6][3]C.6}{[1][39][]39}{}{}{}}
\newlabel{thm:sound-consistency}{{C.6}{39}{Soundness of consistency}{lemma.appendix.C.6}{}}
\newlabel{thm:sound-consistency@cref}{{[lemma][6][3]C.6}{[1][39][]39}{}{}{}}
\newlabel{thmt@@completeConsistency@data}{{\def \theequation {\@arabic {\c@equation }}\def \theHequation {(restate \theHthmt@dummyctr )0}\setcounter {equation}{0}}{39}{Algorithmic Consistency}{Item.8}{}}
\newlabel{thmt@@completeConsistency@data@cref}{{[appendix][6][3]C.6}{[1][39][]39}{}{}{}}
\newlabel{thmt@@completeConsistency}{{C.7}{39}{Completeness and optimality of consistency}{lemma.appendix.C.7}{}}
\newlabel{thmt@@completeConsistency@cref}{{[lemma][7][3]C.7}{[1][39][]39}{}{}{}}
\newlabel{thm:complete-consistency}{{C.7}{39}{Completeness and optimality of consistency}{lemma.appendix.C.7}{}}
\newlabel{thm:complete-consistency@cref}{{[lemma][7][3]C.7}{[1][39][]39}{}{}{}}
\newlabel{fig:alg-consistency}{{19}{40}{Algorithmic consistency}{figure.caption.38}{}}
\newlabel{fig:alg-consistency@cref}{{[figure][19][]19}{[1][39][]40}{}{}{}}
\newlabel{app:proof-algorithm}{{D}{41}{Proofs for Algorithms}{appendix.D}{}}
\newlabel{app:proof-algorithm@cref}{{[appendix][4][]D}{[1][41][]41}{}{}{}}
\newlabel{lemma:suffix-moving}{{D.1}{41}{Suffix moving}{lemma.appendix.D.1}{}}
\newlabel{lemma:suffix-moving@cref}{{[lemma][1][4]D.1}{[1][41][]41}{}{}{}}
\newlabel{lemma:suffix-erasure}{{D.2}{41}{Suffix erasure}{lemma.appendix.D.2}{}}
\newlabel{lemma:suffix-erasure@cref}{{[lemma][2][4]D.2}{[1][41][]41}{}{}{}}
\newlabel{lemma:split-refine}{{D.3}{41}{Splitting refines}{lemma.appendix.D.3}{}}
\newlabel{lemma:split-refine@cref}{{[lemma][3][4]D.3}{[1][41][]41}{}{}{}}
\newlabel{lemma:precision-sub}{{D.4}{41}{Precision extends skeleton subtyping}{lemma.appendix.D.4}{}}
\newlabel{lemma:precision-sub@cref}{{[lemma][4][4]D.4}{[1][41][]41}{}{}{}}
\newlabel{lemma:precision-preserves-refinement}{{D.5}{41}{Precision preserves refinement}{lemma.appendix.D.5}{}}
\newlabel{lemma:precision-preserves-refinement@cref}{{[lemma][5][4]D.5}{[1][41][]41}{}{}{}}
\newlabel{lemma:context-precision-skeleton}{{D.7}{41}{Context precision preserves skeleton inference}{lemma.appendix.D.7}{}}
\newlabel{lemma:context-precision-skeleton@cref}{{[lemma][7][4]D.7}{[1][41][]41}{}{}{}}
\newlabel{app:proof-type-inference}{{D.2}{41}{Type Inference}{subsection.D.2}{}}
\newlabel{app:proof-type-inference@cref}{{[appendix][2][4]D.2}{[1][41][]41}{}{}{}}
\newlabel{app:proof-skeleton-inference}{{D.3}{52}{Skeleton Inference}{subsection.D.3}{}}
\newlabel{app:proof-skeleton-inference@cref}{{[appendix][3][4]D.3}{[1][51][]52}{}{}{}}
\newlabel{app:proof-subtyping}{{E}{60}{Subtyping}{appendix.E}{}}
\newlabel{app:proof-subtyping@cref}{{[appendix][5][]E}{[1][60][]60}{}{}{}}
\newlabel{app:decorated-algosub}{{E.1}{60}{Decorated Algorithmic Judgements}{subsection.E.1}{}}
\newlabel{app:decorated-algosub@cref}{{[appendix][1][5]E.1}{[1][60][]60}{}{}{}}
\newlabel{fig:decorated-alg-subtyping}{{20}{60}{Decorated algorithmic subtyping (only showing non-trivial rules)}{figure.caption.39}{}}
\newlabel{fig:decorated-alg-subtyping@cref}{{[figure][20][]20}{[1][60][]60}{}{}{}}
\newlabel{fig:decorated-alg-consistency}{{21}{61}{Decorated algorithmic consistency}{figure.caption.40}{}}
\newlabel{fig:decorated-alg-consistency@cref}{{[figure][21][]21}{[1][60][]61}{}{}{}}
\newlabel{fig:decorated-tag-solving}{{22}{62}{Decorated tag solving}{figure.caption.41}{}}
\newlabel{fig:decorated-tag-solving@cref}{{[figure][22][]22}{[1][61][]62}{}{}{}}
\newlabel{thmt@@decoratingAlgoSubtyping@data}{{\def \theequation {\@arabic {\c@equation }}\def \theHequation {(restate \theHthmt@dummyctr )0}\setcounter {equation}{0}}{62}{Soundness of Subtyping}{theorem.dummy.40}{}}
\newlabel{thmt@@decoratingAlgoSubtyping@data@cref}{{[appendix][2][5]E.2}{[1][62][]62}{}{}{}}
\newlabel{thmt@@decoratingAlgoSubtyping}{{E.1}{62}{Decorating algorithmic subtyping}{lemma.appendix.E.1}{}}
\newlabel{thmt@@decoratingAlgoSubtyping@cref}{{[lemma][1][5]E.1}{[1][62][]62}{}{}{}}
\newlabel{lemma:decorating-algorithmic-subtyping}{{E.1}{62}{Decorating algorithmic subtyping}{lemma.appendix.E.1}{}}
\newlabel{lemma:decorating-algorithmic-subtyping@cref}{{[lemma][1][5]E.1}{[1][62][]62}{}{}{}}
\newlabel{thmt@@soundDecoratedSubtyping@data}{{\def \theequation {\@arabic {\c@equation }}\def \theHequation {(restate \theHthmt@dummyctr )0}\setcounter {equation}{0}}{62}{Soundness of Subtyping}{lemma.appendix.E.1}{}}
\newlabel{thmt@@soundDecoratedSubtyping@data@cref}{{[appendix][2][5]E.2}{[1][62][]62}{}{}{}}
\newlabel{thmt@@soundDecoratedSubtyping}{{E.2}{62}{Soundness of decorated subtyping}{lemma.appendix.E.2}{}}
\newlabel{thmt@@soundDecoratedSubtyping@cref}{{[lemma][2][5]E.2}{[1][62][]62}{}{}{}}
\newlabel{lemma:sound-decorated-subtyping}{{E.2}{62}{Soundness of decorated subtyping}{lemma.appendix.E.2}{}}
\newlabel{lemma:sound-decorated-subtyping@cref}{{[lemma][2][5]E.2}{[1][62][]62}{}{}{}}
\newlabel{lemma:look-decoration}{{E.3}{63}{Look decoration}{lemma.appendix.E.3}{}}
\newlabel{lemma:look-decoration@cref}{{[lemma][3][5]E.3}{[1][63][]63}{}{}{}}
\newlabel{lemma:decorate-constraint-solving}{{E.4}{63}{Decorating constraint solving}{lemma.appendix.E.4}{}}
\newlabel{lemma:decorate-constraint-solving@cref}{{[lemma][4][5]E.4}{[1][63][]63}{}{}{}}
\newlabel{lemma:solvetag-concat}{{E.5}{63}{Constraint solving concatenation}{lemma.appendix.E.5}{}}
\newlabel{lemma:solvetag-concat@cref}{{[lemma][5][5]E.5}{[1][63][]63}{}{}{}}
\newlabel{lemma:subtyping-decoration-var}{{E.6}{63}{Subtyping decoration for variables}{lemma.appendix.E.6}{}}
\newlabel{lemma:subtyping-decoration-var@cref}{{[lemma][6][5]E.6}{[1][63][]63}{}{}{}}
\newlabel{lemma:vacuous-subtyping-decoration}{{E.7}{66}{Vacuous subtyping decoration}{lemma.appendix.E.7}{}}
\newlabel{lemma:vacuous-subtyping-decoration@cref}{{[lemma][7][5]E.7}{[1][66][]66}{}{}{}}
\newlabel{lemma:constraint-collection-stable-substitution}{{E.8}{66}{Stability of constraint collection}{lemma.appendix.E.8}{}}
\newlabel{lemma:constraint-collection-stable-substitution@cref}{{[lemma][8][5]E.8}{[1][66][]66}{}{}{}}
\newlabel{lemma:look-output-fresh}{{E.9}{66}{Look freshness}{lemma.appendix.E.9}{}}
\newlabel{lemma:look-output-fresh@cref}{{[lemma][9][5]E.9}{[1][66][]66}{}{}{}}
\newlabel{lemma:subtyping-decoration}{{E.10}{67}{Subtyping decoration}{lemma.appendix.E.10}{}}
\newlabel{lemma:subtyping-decoration@cref}{{[lemma][10][5]E.10}{[1][67][]67}{}{}{}}
\newlabel{lemma:look-decoration-replacement}{{E.11}{70}{Decorating instantiation}{lemma.appendix.E.11}{}}
\newlabel{lemma:look-decoration-replacement@cref}{{[lemma][11][5]E.11}{[1][70][]70}{}{}{}}
\newlabel{lemma:sound-decorated-flex-subtyping}{{E.12}{71}{Soundness of decorated algorithmic subtyping of flexible variables}{lemma.appendix.E.12}{}}
\newlabel{lemma:sound-decorated-flex-subtyping@cref}{{[lemma][12][5]E.12}{[1][71][]71}{}{}{}}
\newlabel{lemma:partial-precision-complete}{{E.13}{76}{Complete partial precision}{lemma.appendix.E.13}{}}
\newlabel{lemma:partial-precision-complete@cref}{{[lemma][13][5]E.13}{[1][76][]76}{}{}{}}
\newlabel{lemma:precision-substitution}{{E.14}{76}{Stability of subtyping under more precise substitution}{lemma.appendix.E.14}{}}
\newlabel{lemma:precision-substitution@cref}{{[lemma][14][5]E.14}{[1][76][]76}{}{}{}}
\newlabel{lemma:complete-constraint-collection-solving-var}{{E.15}{76}{Completeness of constraint collection and solving for variables}{lemma.appendix.E.15}{}}
\newlabel{lemma:complete-constraint-collection-solving-var@cref}{{[lemma][15][5]E.15}{[1][76][]76}{}{}{}}
\newlabel{lemma:complete-constraint-collection-solving}{{E.16}{80}{Completeness of constraint collection and solving}{lemma.appendix.E.16}{}}
\newlabel{lemma:complete-constraint-collection-solving@cref}{{[lemma][16][5]E.16}{[1][80][]80}{}{}{}}
\newlabel{lemma:complete-look}{{E.17}{84}{Look completeness}{lemma.appendix.E.17}{}}
\newlabel{lemma:complete-look@cref}{{[lemma][17][5]E.17}{[1][84][]84}{}{}{}}
\newlabel{lemma:complete-flex-subtyping}{{E.18}{85}{Completeness of flexible-variable subtyping}{lemma.appendix.E.18}{}}
\newlabel{lemma:complete-flex-subtyping@cref}{{[lemma][18][5]E.18}{[1][85][]85}{}{}{}}
\newlabel{app:proof-consistency}{{F}{92}{Consistency}{appendix.F}{}}
\newlabel{app:proof-consistency@cref}{{[appendix][6][]F}{[1][92][]92}{}{}{}}
\newlabel{lemma:sound-decorated-consistency}{{F.1}{92}{Soundness of decorated consistency}{lemma.appendix.F.1}{}}
\newlabel{lemma:sound-decorated-consistency@cref}{{[lemma][1][6]F.1}{[1][92][]92}{}{}{}}
\newlabel{lemma:decorating-algorithmic-consistency}{{F.2}{92}{Decorating algorithmic consistency}{lemma.appendix.F.2}{}}
\newlabel{lemma:decorating-algorithmic-consistency@cref}{{[lemma][2][6]F.2}{[1][92][]92}{}{}{}}
\newlabel{lemma:consistency-decoration}{{F.3}{92}{Consistency decoration}{lemma.appendix.F.3}{}}
\newlabel{lemma:consistency-decoration@cref}{{[lemma][3][6]F.3}{[1][92][]92}{}{}{}}
\newlabel{lemma:consistency-decoration-var}{{F.4}{97}{Consistency constraint decoration for variables}{lemma.appendix.F.4}{}}
\newlabel{lemma:consistency-decoration-var@cref}{{[lemma][4][6]F.4}{[1][97][]97}{}{}{}}
\newlabel{lemma:complete-consistency-constraint-collection-solving}{{F.5}{100}{Completeness of consistency constraint collection and solving}{lemma.appendix.F.5}{}}
\newlabel{lemma:complete-consistency-constraint-collection-solving@cref}{{[lemma][5][6]F.5}{[1][100][]100}{}{}{}}
\newlabel{lemma:complete-consistency-constraint-collection-solving-var}{{F.6}{102}{Completeness of consistency constraint collection and solving for variables}{lemma.appendix.F.6}{}}
\newlabel{lemma:complete-consistency-constraint-collection-solving-var@cref}{{[lemma][6][6]F.6}{[1][102][]102}{}{}{}}
\newlabel{app:proof-sound-consistency}{{F.2}{105}{Soundness of Consistency}{subsection.F.2}{}}
\newlabel{app:proof-sound-consistency@cref}{{[appendix][2][6]F.2}{[1][105][]105}{}{}{}}
\newcommand{\AppendixPDFAnchor}[1]{%
  \Hy@raisedlink{%
    \hyper@anchorstart{#1}\hyper@anchorend%
  }%
}
\PAX@DestProv{appendix.pax}{39}
\PAX@DestProv{appendix.pax}{123}
\PAX@DestProv{appendix.pax}{154}
\PAX@DestProv{appendix.pax}{159}
\expandafter\def\csname AppendixMainAnchors@1\endcsname{\AppendixPDFAnchor{PAX@appendix.pax@39}\AppendixPDFAnchor{PAX@appendix.pax@123}\AppendixPDFAnchor{PAX@appendix.pax@154}\AppendixPDFAnchor{PAX@appendix.pax@159}}
\PAX@DestProv{appendix.pax}{20}
\PAX@DestProv{appendix.pax}{26}
\expandafter\def\csname AppendixMainAnchors@2\endcsname{\AppendixPDFAnchor{PAX@appendix.pax@20}\AppendixPDFAnchor{PAX@appendix.pax@26}}
\PAX@DestProv{appendix.pax}{33}
\PAX@DestProv{appendix.pax}{47}
\PAX@DestProv{appendix.pax}{53}
\PAX@DestProv{appendix.pax}{56}
\PAX@DestProv{appendix.pax}{58}
\expandafter\def\csname AppendixMainAnchors@3\endcsname{\AppendixPDFAnchor{PAX@appendix.pax@33}\AppendixPDFAnchor{PAX@appendix.pax@47}\AppendixPDFAnchor{PAX@appendix.pax@53}\AppendixPDFAnchor{PAX@appendix.pax@56}\AppendixPDFAnchor{PAX@appendix.pax@58}}
\PAX@DestProv{appendix.pax}{65}
\expandafter\def\csname AppendixMainAnchors@4\endcsname{\AppendixPDFAnchor{PAX@appendix.pax@65}}
\PAX@DestProv{appendix.pax}{71}
\PAX@DestProv{appendix.pax}{72}
\PAX@DestProv{appendix.pax}{77}
\PAX@DestProv{appendix.pax}{90}
\expandafter\def\csname AppendixMainAnchors@5\endcsname{\AppendixPDFAnchor{PAX@appendix.pax@71}\AppendixPDFAnchor{PAX@appendix.pax@72}\AppendixPDFAnchor{PAX@appendix.pax@77}\AppendixPDFAnchor{PAX@appendix.pax@90}}
\PAX@DestProv{appendix.pax}{66}
\PAX@DestProv{appendix.pax}{79}
\PAX@DestProv{appendix.pax}{87}
\PAX@DestProv{appendix.pax}{89}
\PAX@DestProv{appendix.pax}{162}
\expandafter\def\csname AppendixMainAnchors@6\endcsname{\AppendixPDFAnchor{PAX@appendix.pax@66}\AppendixPDFAnchor{PAX@appendix.pax@79}\AppendixPDFAnchor{PAX@appendix.pax@87}\AppendixPDFAnchor{PAX@appendix.pax@89}\AppendixPDFAnchor{PAX@appendix.pax@162}}
\PAX@DestProv{appendix.pax}{82}
\expandafter\def\csname AppendixMainAnchors@8\endcsname{\AppendixPDFAnchor{PAX@appendix.pax@82}}
\PAX@DestProv{appendix.pax}{181}
\expandafter\def\csname AppendixMainAnchors@9\endcsname{\AppendixPDFAnchor{PAX@appendix.pax@181}}
\PAX@DestProv{appendix.pax}{34}
\PAX@DestProv{appendix.pax}{102}
\PAX@DestProv{appendix.pax}{106}
\PAX@DestProv{appendix.pax}{109}
\PAX@DestProv{appendix.pax}{145}
\PAX@DestProv{appendix.pax}{204}
\PAX@DestProv{appendix.pax}{209}
\PAX@DestProv{appendix.pax}{212}
\expandafter\def\csname AppendixMainAnchors@10\endcsname{\AppendixPDFAnchor{PAX@appendix.pax@34}\AppendixPDFAnchor{PAX@appendix.pax@102}\AppendixPDFAnchor{PAX@appendix.pax@106}\AppendixPDFAnchor{PAX@appendix.pax@109}\AppendixPDFAnchor{PAX@appendix.pax@145}\AppendixPDFAnchor{PAX@appendix.pax@204}\AppendixPDFAnchor{PAX@appendix.pax@209}\AppendixPDFAnchor{PAX@appendix.pax@212}}
\PAX@DestProv{appendix.pax}{76}
\PAX@DestProv{appendix.pax}{83}
\PAX@DestProv{appendix.pax}{92}
\PAX@DestProv{appendix.pax}{115}
\PAX@DestProv{appendix.pax}{117}
\PAX@DestProv{appendix.pax}{147}
\expandafter\def\csname AppendixMainAnchors@11\endcsname{\AppendixPDFAnchor{PAX@appendix.pax@76}\AppendixPDFAnchor{PAX@appendix.pax@83}\AppendixPDFAnchor{PAX@appendix.pax@92}\AppendixPDFAnchor{PAX@appendix.pax@115}\AppendixPDFAnchor{PAX@appendix.pax@117}\AppendixPDFAnchor{PAX@appendix.pax@147}}
\PAX@DestProv{appendix.pax}{78}
\PAX@DestProv{appendix.pax}{93}
\PAX@DestProv{appendix.pax}{94}
\PAX@DestProv{appendix.pax}{95}
\PAX@DestProv{appendix.pax}{96}
\PAX@DestProv{appendix.pax}{114}
\PAX@DestProv{appendix.pax}{116}
\PAX@DestProv{appendix.pax}{138}
\PAX@DestProv{appendix.pax}{146}
\PAX@DestProv{appendix.pax}{177}
\PAX@DestProv{appendix.pax}{213}
\PAX@DestProv{appendix.pax}{223}
\PAX@DestProv{appendix.pax}{226}
\expandafter\def\csname AppendixMainAnchors@12\endcsname{\AppendixPDFAnchor{PAX@appendix.pax@78}\AppendixPDFAnchor{PAX@appendix.pax@93}\AppendixPDFAnchor{PAX@appendix.pax@94}\AppendixPDFAnchor{PAX@appendix.pax@95}\AppendixPDFAnchor{PAX@appendix.pax@96}\AppendixPDFAnchor{PAX@appendix.pax@114}\AppendixPDFAnchor{PAX@appendix.pax@116}\AppendixPDFAnchor{PAX@appendix.pax@138}\AppendixPDFAnchor{PAX@appendix.pax@146}\AppendixPDFAnchor{PAX@appendix.pax@177}\AppendixPDFAnchor{PAX@appendix.pax@213}\AppendixPDFAnchor{PAX@appendix.pax@223}\AppendixPDFAnchor{PAX@appendix.pax@226}}
\PAX@DestProv{appendix.pax}{88}
\PAX@DestProv{appendix.pax}{98}
\PAX@DestProv{appendix.pax}{100}
\PAX@DestProv{appendix.pax}{101}
\expandafter\def\csname AppendixMainAnchors@13\endcsname{\AppendixPDFAnchor{PAX@appendix.pax@88}\AppendixPDFAnchor{PAX@appendix.pax@98}\AppendixPDFAnchor{PAX@appendix.pax@100}\AppendixPDFAnchor{PAX@appendix.pax@101}}
\PAX@DestProv{appendix.pax}{80}
\PAX@DestProv{appendix.pax}{111}
\expandafter\def\csname AppendixMainAnchors@14\endcsname{\AppendixPDFAnchor{PAX@appendix.pax@80}\AppendixPDFAnchor{PAX@appendix.pax@111}}
\PAX@DestProv{appendix.pax}{48}
\PAX@DestProv{appendix.pax}{81}
\PAX@DestProv{appendix.pax}{85}
\PAX@DestProv{appendix.pax}{91}
\PAX@DestProv{appendix.pax}{121}
\PAX@DestProv{appendix.pax}{124}
\PAX@DestProv{appendix.pax}{131}
\PAX@DestProv{appendix.pax}{139}
\PAX@DestProv{appendix.pax}{148}
\PAX@DestProv{appendix.pax}{220}
\PAX@DestProv{appendix.pax}{222}
\PAX@DestProv{appendix.pax}{227}
\expandafter\def\csname AppendixMainAnchors@15\endcsname{\AppendixPDFAnchor{PAX@appendix.pax@48}\AppendixPDFAnchor{PAX@appendix.pax@81}\AppendixPDFAnchor{PAX@appendix.pax@85}\AppendixPDFAnchor{PAX@appendix.pax@91}\AppendixPDFAnchor{PAX@appendix.pax@121}\AppendixPDFAnchor{PAX@appendix.pax@124}\AppendixPDFAnchor{PAX@appendix.pax@131}\AppendixPDFAnchor{PAX@appendix.pax@139}\AppendixPDFAnchor{PAX@appendix.pax@148}\AppendixPDFAnchor{PAX@appendix.pax@220}\AppendixPDFAnchor{PAX@appendix.pax@222}\AppendixPDFAnchor{PAX@appendix.pax@227}}
\PAX@DestProv{appendix.pax}{97}
\PAX@DestProv{appendix.pax}{206}
\PAX@DestProv{appendix.pax}{235}
\expandafter\def\csname AppendixMainAnchors@16\endcsname{\AppendixPDFAnchor{PAX@appendix.pax@97}\AppendixPDFAnchor{PAX@appendix.pax@206}\AppendixPDFAnchor{PAX@appendix.pax@235}}
\PAX@DestProv{appendix.pax}{35}
\PAX@DestProv{appendix.pax}{86}
\PAX@DestProv{appendix.pax}{207}
\expandafter\def\csname AppendixMainAnchors@17\endcsname{\AppendixPDFAnchor{PAX@appendix.pax@35}\AppendixPDFAnchor{PAX@appendix.pax@86}\AppendixPDFAnchor{PAX@appendix.pax@207}}
\PAX@DestProv{appendix.pax}{112}
\PAX@DestProv{appendix.pax}{122}
\PAX@DestProv{appendix.pax}{125}
\PAX@DestProv{appendix.pax}{140}
\PAX@DestProv{appendix.pax}{216}
\PAX@DestProv{appendix.pax}{237}
\expandafter\def\csname AppendixMainAnchors@18\endcsname{\AppendixPDFAnchor{PAX@appendix.pax@112}\AppendixPDFAnchor{PAX@appendix.pax@122}\AppendixPDFAnchor{PAX@appendix.pax@125}\AppendixPDFAnchor{PAX@appendix.pax@140}\AppendixPDFAnchor{PAX@appendix.pax@216}\AppendixPDFAnchor{PAX@appendix.pax@237}}
\PAX@DestProv{appendix.pax}{126}
\PAX@DestProv{appendix.pax}{224}
\expandafter\def\csname AppendixMainAnchors@19\endcsname{\AppendixPDFAnchor{PAX@appendix.pax@126}\AppendixPDFAnchor{PAX@appendix.pax@224}}
\PAX@DestProv{appendix.pax}{129}
\expandafter\def\csname AppendixMainAnchors@20\endcsname{\AppendixPDFAnchor{PAX@appendix.pax@129}}
\PAX@DestProv{appendix.pax}{105}
\PAX@DestProv{appendix.pax}{228}
\PAX@DestProv{appendix.pax}{232}
\expandafter\def\csname AppendixMainAnchors@21\endcsname{\AppendixPDFAnchor{PAX@appendix.pax@105}\AppendixPDFAnchor{PAX@appendix.pax@228}\AppendixPDFAnchor{PAX@appendix.pax@232}}
\PAX@DestProv{appendix.pax}{137}
\expandafter\def\csname AppendixMainAnchors@22\endcsname{\AppendixPDFAnchor{PAX@appendix.pax@137}}
\PAX@DestProv{appendix.pax}{36}
\PAX@DestProv{appendix.pax}{69}
\PAX@DestProv{appendix.pax}{239}
\PAX@DestProv{appendix.pax}{240}
\PAX@DestProv{appendix.pax}{241}
\PAX@DestProv{appendix.pax}{254}
\PAX@DestProv{appendix.pax}{261}
\PAX@DestProv{appendix.pax}{262}
\PAX@DestProv{appendix.pax}{263}
\PAX@DestProv{appendix.pax}{268}
\PAX@DestProv{appendix.pax}{278}
\PAX@DestProv{appendix.pax}{317}
\PAX@DestProv{appendix.pax}{318}
\PAX@DestProv{appendix.pax}{319}
\expandafter\def\csname AppendixMainAnchors@23\endcsname{\AppendixPDFAnchor{PAX@appendix.pax@36}\AppendixPDFAnchor{PAX@appendix.pax@69}\AppendixPDFAnchor{PAX@appendix.pax@239}\AppendixPDFAnchor{PAX@appendix.pax@240}\AppendixPDFAnchor{PAX@appendix.pax@241}\AppendixPDFAnchor{PAX@appendix.pax@254}\AppendixPDFAnchor{PAX@appendix.pax@261}\AppendixPDFAnchor{PAX@appendix.pax@262}\AppendixPDFAnchor{PAX@appendix.pax@263}\AppendixPDFAnchor{PAX@appendix.pax@268}\AppendixPDFAnchor{PAX@appendix.pax@278}\AppendixPDFAnchor{PAX@appendix.pax@317}\AppendixPDFAnchor{PAX@appendix.pax@318}\AppendixPDFAnchor{PAX@appendix.pax@319}}
\PAX@DestProv{appendix.pax}{38}
\expandafter\def\csname AppendixMainAnchors@24\endcsname{\AppendixPDFAnchor{PAX@appendix.pax@38}}
\PAX@DestProv{appendix.pax}{1}
\PAX@DestProv{appendix.pax}{3}
\PAX@DestProv{appendix.pax}{7}
\PAX@DestProv{appendix.pax}{15}
\PAX@DestProv{appendix.pax}{27}
\PAX@DestProv{appendix.pax}{28}
\PAX@DestProv{appendix.pax}{29}
\PAX@DestProv{appendix.pax}{40}
\PAX@DestProv{appendix.pax}{41}
\PAX@DestProv{appendix.pax}{42}
\PAX@DestProv{appendix.pax}{45}
\PAX@DestProv{appendix.pax}{59}
\PAX@DestProv{appendix.pax}{61}
\PAX@DestProv{appendix.pax}{62}
\PAX@DestProv{appendix.pax}{70}
\PAX@DestProv{appendix.pax}{73}
\PAX@DestProv{appendix.pax}{144}
\PAX@DestProv{appendix.pax}{171}
\PAX@DestProv{appendix.pax}{175}
\PAX@DestProv{appendix.pax}{178}
\PAX@DestProv{appendix.pax}{184}
\expandafter\def\csname AppendixMainAnchors@26\endcsname{\AppendixPDFAnchor{PAX@appendix.pax@1}\AppendixPDFAnchor{PAX@appendix.pax@3}\AppendixPDFAnchor{PAX@appendix.pax@7}\AppendixPDFAnchor{PAX@appendix.pax@15}\AppendixPDFAnchor{PAX@appendix.pax@27}\AppendixPDFAnchor{PAX@appendix.pax@28}\AppendixPDFAnchor{PAX@appendix.pax@29}\AppendixPDFAnchor{PAX@appendix.pax@40}\AppendixPDFAnchor{PAX@appendix.pax@41}\AppendixPDFAnchor{PAX@appendix.pax@42}\AppendixPDFAnchor{PAX@appendix.pax@45}\AppendixPDFAnchor{PAX@appendix.pax@59}\AppendixPDFAnchor{PAX@appendix.pax@61}\AppendixPDFAnchor{PAX@appendix.pax@62}\AppendixPDFAnchor{PAX@appendix.pax@70}\AppendixPDFAnchor{PAX@appendix.pax@73}\AppendixPDFAnchor{PAX@appendix.pax@144}\AppendixPDFAnchor{PAX@appendix.pax@171}\AppendixPDFAnchor{PAX@appendix.pax@175}\AppendixPDFAnchor{PAX@appendix.pax@178}\AppendixPDFAnchor{PAX@appendix.pax@184}}
\PAX@DestProv{appendix.pax}{2}
\PAX@DestProv{appendix.pax}{4}
\PAX@DestProv{appendix.pax}{5}
\PAX@DestProv{appendix.pax}{6}
\PAX@DestProv{appendix.pax}{8}
\PAX@DestProv{appendix.pax}{10}
\PAX@DestProv{appendix.pax}{11}
\PAX@DestProv{appendix.pax}{12}
\PAX@DestProv{appendix.pax}{13}
\PAX@DestProv{appendix.pax}{14}
\PAX@DestProv{appendix.pax}{16}
\PAX@DestProv{appendix.pax}{17}
\PAX@DestProv{appendix.pax}{19}
\PAX@DestProv{appendix.pax}{21}
\PAX@DestProv{appendix.pax}{22}
\PAX@DestProv{appendix.pax}{23}
\PAX@DestProv{appendix.pax}{30}
\PAX@DestProv{appendix.pax}{31}
\PAX@DestProv{appendix.pax}{43}
\PAX@DestProv{appendix.pax}{51}
\PAX@DestProv{appendix.pax}{52}
\PAX@DestProv{appendix.pax}{54}
\PAX@DestProv{appendix.pax}{55}
\PAX@DestProv{appendix.pax}{60}
\PAX@DestProv{appendix.pax}{63}
\PAX@DestProv{appendix.pax}{67}
\PAX@DestProv{appendix.pax}{74}
\PAX@DestProv{appendix.pax}{103}
\PAX@DestProv{appendix.pax}{104}
\PAX@DestProv{appendix.pax}{107}
\PAX@DestProv{appendix.pax}{118}
\PAX@DestProv{appendix.pax}{132}
\PAX@DestProv{appendix.pax}{149}
\PAX@DestProv{appendix.pax}{150}
\PAX@DestProv{appendix.pax}{156}
\PAX@DestProv{appendix.pax}{157}
\PAX@DestProv{appendix.pax}{158}
\PAX@DestProv{appendix.pax}{160}
\PAX@DestProv{appendix.pax}{161}
\PAX@DestProv{appendix.pax}{165}
\PAX@DestProv{appendix.pax}{166}
\PAX@DestProv{appendix.pax}{167}
\PAX@DestProv{appendix.pax}{168}
\PAX@DestProv{appendix.pax}{169}
\PAX@DestProv{appendix.pax}{170}
\PAX@DestProv{appendix.pax}{172}
\PAX@DestProv{appendix.pax}{173}
\PAX@DestProv{appendix.pax}{174}
\PAX@DestProv{appendix.pax}{179}
\PAX@DestProv{appendix.pax}{182}
\PAX@DestProv{appendix.pax}{183}
\PAX@DestProv{appendix.pax}{185}
\PAX@DestProv{appendix.pax}{186}
\PAX@DestProv{appendix.pax}{188}
\PAX@DestProv{appendix.pax}{189}
\PAX@DestProv{appendix.pax}{192}
\PAX@DestProv{appendix.pax}{193}
\PAX@DestProv{appendix.pax}{194}
\PAX@DestProv{appendix.pax}{195}
\PAX@DestProv{appendix.pax}{196}
\PAX@DestProv{appendix.pax}{197}
\PAX@DestProv{appendix.pax}{198}
\PAX@DestProv{appendix.pax}{199}
\PAX@DestProv{appendix.pax}{200}
\PAX@DestProv{appendix.pax}{201}
\PAX@DestProv{appendix.pax}{202}
\PAX@DestProv{appendix.pax}{203}
\expandafter\def\csname AppendixMainAnchors@27\endcsname{\AppendixPDFAnchor{PAX@appendix.pax@2}\AppendixPDFAnchor{PAX@appendix.pax@4}\AppendixPDFAnchor{PAX@appendix.pax@5}\AppendixPDFAnchor{PAX@appendix.pax@6}\AppendixPDFAnchor{PAX@appendix.pax@8}\AppendixPDFAnchor{PAX@appendix.pax@10}\AppendixPDFAnchor{PAX@appendix.pax@11}\AppendixPDFAnchor{PAX@appendix.pax@12}\AppendixPDFAnchor{PAX@appendix.pax@13}\AppendixPDFAnchor{PAX@appendix.pax@14}\AppendixPDFAnchor{PAX@appendix.pax@16}\AppendixPDFAnchor{PAX@appendix.pax@17}\AppendixPDFAnchor{PAX@appendix.pax@19}\AppendixPDFAnchor{PAX@appendix.pax@21}\AppendixPDFAnchor{PAX@appendix.pax@22}\AppendixPDFAnchor{PAX@appendix.pax@23}\AppendixPDFAnchor{PAX@appendix.pax@30}\AppendixPDFAnchor{PAX@appendix.pax@31}\AppendixPDFAnchor{PAX@appendix.pax@43}\AppendixPDFAnchor{PAX@appendix.pax@51}\AppendixPDFAnchor{PAX@appendix.pax@52}\AppendixPDFAnchor{PAX@appendix.pax@54}\AppendixPDFAnchor{PAX@appendix.pax@55}\AppendixPDFAnchor{PAX@appendix.pax@60}\AppendixPDFAnchor{PAX@appendix.pax@63}\AppendixPDFAnchor{PAX@appendix.pax@67}\AppendixPDFAnchor{PAX@appendix.pax@74}\AppendixPDFAnchor{PAX@appendix.pax@103}\AppendixPDFAnchor{PAX@appendix.pax@104}\AppendixPDFAnchor{PAX@appendix.pax@107}\AppendixPDFAnchor{PAX@appendix.pax@118}\AppendixPDFAnchor{PAX@appendix.pax@132}\AppendixPDFAnchor{PAX@appendix.pax@149}\AppendixPDFAnchor{PAX@appendix.pax@150}\AppendixPDFAnchor{PAX@appendix.pax@156}\AppendixPDFAnchor{PAX@appendix.pax@157}\AppendixPDFAnchor{PAX@appendix.pax@158}\AppendixPDFAnchor{PAX@appendix.pax@160}\AppendixPDFAnchor{PAX@appendix.pax@161}\AppendixPDFAnchor{PAX@appendix.pax@165}\AppendixPDFAnchor{PAX@appendix.pax@166}\AppendixPDFAnchor{PAX@appendix.pax@167}\AppendixPDFAnchor{PAX@appendix.pax@168}\AppendixPDFAnchor{PAX@appendix.pax@169}\AppendixPDFAnchor{PAX@appendix.pax@170}\AppendixPDFAnchor{PAX@appendix.pax@172}\AppendixPDFAnchor{PAX@appendix.pax@173}\AppendixPDFAnchor{PAX@appendix.pax@174}\AppendixPDFAnchor{PAX@appendix.pax@179}\AppendixPDFAnchor{PAX@appendix.pax@182}\AppendixPDFAnchor{PAX@appendix.pax@183}\AppendixPDFAnchor{PAX@appendix.pax@185}\AppendixPDFAnchor{PAX@appendix.pax@186}\AppendixPDFAnchor{PAX@appendix.pax@188}\AppendixPDFAnchor{PAX@appendix.pax@189}\AppendixPDFAnchor{PAX@appendix.pax@192}\AppendixPDFAnchor{PAX@appendix.pax@193}\AppendixPDFAnchor{PAX@appendix.pax@194}\AppendixPDFAnchor{PAX@appendix.pax@195}\AppendixPDFAnchor{PAX@appendix.pax@196}\AppendixPDFAnchor{PAX@appendix.pax@197}\AppendixPDFAnchor{PAX@appendix.pax@198}\AppendixPDFAnchor{PAX@appendix.pax@199}\AppendixPDFAnchor{PAX@appendix.pax@200}\AppendixPDFAnchor{PAX@appendix.pax@201}\AppendixPDFAnchor{PAX@appendix.pax@202}\AppendixPDFAnchor{PAX@appendix.pax@203}}
\PAX@DestProv{appendix.pax}{9}
\PAX@DestProv{appendix.pax}{18}
\PAX@DestProv{appendix.pax}{24}
\PAX@DestProv{appendix.pax}{25}
\PAX@DestProv{appendix.pax}{37}
\PAX@DestProv{appendix.pax}{44}
\PAX@DestProv{appendix.pax}{46}
\PAX@DestProv{appendix.pax}{49}
\PAX@DestProv{appendix.pax}{50}
\PAX@DestProv{appendix.pax}{57}
\PAX@DestProv{appendix.pax}{64}
\PAX@DestProv{appendix.pax}{68}
\PAX@DestProv{appendix.pax}{75}
\PAX@DestProv{appendix.pax}{142}
\PAX@DestProv{appendix.pax}{143}
\PAX@DestProv{appendix.pax}{151}
\PAX@DestProv{appendix.pax}{152}
\PAX@DestProv{appendix.pax}{153}
\PAX@DestProv{appendix.pax}{155}
\PAX@DestProv{appendix.pax}{163}
\PAX@DestProv{appendix.pax}{164}
\PAX@DestProv{appendix.pax}{176}
\PAX@DestProv{appendix.pax}{180}
\expandafter\def\csname AppendixMainAnchors@28\endcsname{\AppendixPDFAnchor{PAX@appendix.pax@9}\AppendixPDFAnchor{PAX@appendix.pax@18}\AppendixPDFAnchor{PAX@appendix.pax@24}\AppendixPDFAnchor{PAX@appendix.pax@25}\AppendixPDFAnchor{PAX@appendix.pax@37}\AppendixPDFAnchor{PAX@appendix.pax@44}\AppendixPDFAnchor{PAX@appendix.pax@46}\AppendixPDFAnchor{PAX@appendix.pax@49}\AppendixPDFAnchor{PAX@appendix.pax@50}\AppendixPDFAnchor{PAX@appendix.pax@57}\AppendixPDFAnchor{PAX@appendix.pax@64}\AppendixPDFAnchor{PAX@appendix.pax@68}\AppendixPDFAnchor{PAX@appendix.pax@75}\AppendixPDFAnchor{PAX@appendix.pax@142}\AppendixPDFAnchor{PAX@appendix.pax@143}\AppendixPDFAnchor{PAX@appendix.pax@151}\AppendixPDFAnchor{PAX@appendix.pax@152}\AppendixPDFAnchor{PAX@appendix.pax@153}\AppendixPDFAnchor{PAX@appendix.pax@155}\AppendixPDFAnchor{PAX@appendix.pax@163}\AppendixPDFAnchor{PAX@appendix.pax@164}\AppendixPDFAnchor{PAX@appendix.pax@176}\AppendixPDFAnchor{PAX@appendix.pax@180}}
\AddToHook{shipout/foreground}{%
  \put(0,0){%
    \@ifundefined{AppendixMainAnchors@\arabic{page}}{}{%
      \csname AppendixMainAnchors@\arabic{page}\endcsname%
    }%
  }%
}
\expandafter\def\csname AppendixPageAnchors@1\endcsname{\AppendixPDFAnchor{appendix.A}\AppendixPDFAnchor{figure.caption.27}}
\expandafter\def\csname AppendixPageAnchors@2\endcsname{\AppendixPDFAnchor{figure.caption.28}\AppendixPDFAnchor{figure.caption.29}}
\expandafter\def\csname AppendixPageAnchors@3\endcsname{\AppendixPDFAnchor{appendix.B}\AppendixPDFAnchor{figure.caption.30}\AppendixPDFAnchor{lemma.appendix.B.1}\AppendixPDFAnchor{lemma.appendix.B.2}\AppendixPDFAnchor{subsection.B.1}\AppendixPDFAnchor{subsection.B.2}}
\expandafter\def\csname AppendixPageAnchors@4\endcsname{\AppendixPDFAnchor{appendix.C}\AppendixPDFAnchor{figure.caption.31}\AppendixPDFAnchor{subsection.C.1}\AppendixPDFAnchor{subsection.C.2}}
\expandafter\def\csname AppendixPageAnchors@5\endcsname{\AppendixPDFAnchor{figure.caption.32}\AppendixPDFAnchor{subsection.C.3}}
\expandafter\def\csname AppendixPageAnchors@6\endcsname{\AppendixPDFAnchor{figure.caption.33}\AppendixPDFAnchor{subsection.C.4}}
\expandafter\def\csname AppendixPageAnchors@7\endcsname{\AppendixPDFAnchor{figure.caption.34}\AppendixPDFAnchor{subsection.C.5}\AppendixPDFAnchor{theorem.appendix.C.2}\AppendixPDFAnchor{theorem.appendix.C.3}}
\expandafter\def\csname AppendixPageAnchors@8\endcsname{\AppendixPDFAnchor{figure.caption.35}}
\expandafter\def\csname AppendixPageAnchors@9\endcsname{\AppendixPDFAnchor{figure.caption.36}}
\expandafter\def\csname AppendixPageAnchors@10\endcsname{\AppendixPDFAnchor{figure.caption.37}\AppendixPDFAnchor{subsection.C.6}}
\expandafter\def\csname AppendixPageAnchors@11\endcsname{\AppendixPDFAnchor{lemma.appendix.C.6}\AppendixPDFAnchor{lemma.appendix.C.7}}
\expandafter\def\csname AppendixPageAnchors@12\endcsname{\AppendixPDFAnchor{figure.caption.38}}
\expandafter\def\csname AppendixPageAnchors@13\endcsname{\AppendixPDFAnchor{appendix.D}\AppendixPDFAnchor{lemma.appendix.D.1}\AppendixPDFAnchor{lemma.appendix.D.2}\AppendixPDFAnchor{lemma.appendix.D.3}\AppendixPDFAnchor{lemma.appendix.D.4}\AppendixPDFAnchor{lemma.appendix.D.5}\AppendixPDFAnchor{lemma.appendix.D.7}\AppendixPDFAnchor{subsection.D.2}}
\expandafter\def\csname AppendixPageAnchors@24\endcsname{\AppendixPDFAnchor{subsection.D.3}}
\expandafter\def\csname AppendixPageAnchors@32\endcsname{\AppendixPDFAnchor{appendix.E}\AppendixPDFAnchor{figure.caption.39}\AppendixPDFAnchor{subsection.E.1}}
\expandafter\def\csname AppendixPageAnchors@33\endcsname{\AppendixPDFAnchor{figure.caption.40}}
\expandafter\def\csname AppendixPageAnchors@34\endcsname{\AppendixPDFAnchor{figure.caption.41}\AppendixPDFAnchor{lemma.appendix.E.1}\AppendixPDFAnchor{lemma.appendix.E.2}}
\expandafter\def\csname AppendixPageAnchors@35\endcsname{\AppendixPDFAnchor{lemma.appendix.E.3}\AppendixPDFAnchor{lemma.appendix.E.4}\AppendixPDFAnchor{lemma.appendix.E.5}\AppendixPDFAnchor{lemma.appendix.E.6}}
\expandafter\def\csname AppendixPageAnchors@38\endcsname{\AppendixPDFAnchor{lemma.appendix.E.7}\AppendixPDFAnchor{lemma.appendix.E.8}\AppendixPDFAnchor{lemma.appendix.E.9}}
\expandafter\def\csname AppendixPageAnchors@39\endcsname{\AppendixPDFAnchor{lemma.appendix.E.10}}
\expandafter\def\csname AppendixPageAnchors@42\endcsname{\AppendixPDFAnchor{lemma.appendix.E.11}}
\expandafter\def\csname AppendixPageAnchors@43\endcsname{\AppendixPDFAnchor{lemma.appendix.E.12}}
\expandafter\def\csname AppendixPageAnchors@48\endcsname{\AppendixPDFAnchor{lemma.appendix.E.13}\AppendixPDFAnchor{lemma.appendix.E.14}\AppendixPDFAnchor{lemma.appendix.E.15}}
\expandafter\def\csname AppendixPageAnchors@52\endcsname{\AppendixPDFAnchor{lemma.appendix.E.16}}
\expandafter\def\csname AppendixPageAnchors@56\endcsname{\AppendixPDFAnchor{lemma.appendix.E.17}}
\expandafter\def\csname AppendixPageAnchors@57\endcsname{\AppendixPDFAnchor{lemma.appendix.E.18}}
\expandafter\def\csname AppendixPageAnchors@64\endcsname{\AppendixPDFAnchor{appendix.F}\AppendixPDFAnchor{lemma.appendix.F.1}\AppendixPDFAnchor{lemma.appendix.F.2}\AppendixPDFAnchor{lemma.appendix.F.3}}
\expandafter\def\csname AppendixPageAnchors@69\endcsname{\AppendixPDFAnchor{lemma.appendix.F.4}}
\expandafter\def\csname AppendixPageAnchors@72\endcsname{\AppendixPDFAnchor{lemma.appendix.F.5}}
\expandafter\def\csname AppendixPageAnchors@74\endcsname{\AppendixPDFAnchor{lemma.appendix.F.6}}
\expandafter\def\csname AppendixPageAnchors@77\endcsname{\AppendixPDFAnchor{subsection.F.2}}
\newcounter{appendixpdfpage}
\newcommand{\AppendixPDFPageCommand}{%
  \thispagestyle{empty}%
  \stepcounter{appendixpdfpage}%
  \@ifundefined{AppendixPageAnchors@\arabic{appendixpdfpage}}{}{%
    \csname AppendixPageAnchors@\arabic{appendixpdfpage}\endcsname%
  }%
}
\makeatother
